# Supplementary material for: GLL-based Context-Free Path Querying for Neo4j
Source: arXiv:2312.11925 source file (2023-12-19)
Supplement: Supplementary file 1 [file appendix.tex]

\begin{lstlisting}[language=caml, caption=Python example]
let handleDescriptor (currentDescriptor:Descriptor) =
    gss.AddDescriptorToHandled currentDescriptor
    if query.IsFinalState currentDescriptor.RSMState                        
    then
        let matchedRange =
            match currentDescriptor.MatchedRange with             
            | None ->
                let newRange =
                    MatchedRange(
                           currentDescriptor.InputPosition
                         , currentDescriptor.InputPosition
                         , currentDescriptor.RSMState
                         , currentDescriptor.RSMState
                         , RangeType.EpsilonNonTerminal currentDescriptor.GSSVertex.RSMState
                    )
                matchedRanges.AddMatchedRange(None, newRange) |> ignore
                newRange
            | Some range -> range
                                            
        gss.Pop(currentDescriptor, matchedRange)            
        |> ResizeArray.iter (
            fun gssEdge ->                
                let leftSubRange = gssEdge.Info
                let rightSubRange =           
                    MatchedRange(
                        currentDescriptor.GSSVertex.InputPosition
                      , currentDescriptor.InputPosition
                      , match gssEdge.Info with
                        | None -> gssEdge.GSSVertex.RSMState
                        | Some v -> v.RSMRange.EndPosition
                      , gssEdge.RSMState
                      , RangeType.NonTerminal currentDescriptor.GSSVertex.RSMState
                    )
                    
                let newRange = matchedRanges.AddMatchedRange(leftSubRange, rightSubRange)
                Descriptor(currentDescriptor.InputPosition, gssEdge.GSSVertex, gssEdge.RSMState, Some newRange)
                |> addDescriptor
            )
        
    let outgoingTerminalEdgesInGraph = graph.OutgoingTerminalEdges currentDescriptor.InputPosition        
    let outgoingNonTerminalEdgesInRSM = query.OutgoingNonTerminalEdges currentDescriptor.RSMState
    let outgoingTerminalEdgesInRSM = query.OutgoingTerminalEdges currentDescriptor.RSMState       
    
    outgoingNonTerminalEdgesInRSM
    |> Array.iter (fun edge ->
           let edge = unpackRSMNonTerminalEdge edge
           let newGSSVertex, positionsForPops =
                gss.AddEdge(currentDescriptor.GSSVertex
                            , edge.State
                            , currentDescriptor.InputPosition
                            , edge.NonTerminalSymbolStartState
                            , currentDescriptor.MatchedRange)
           
           Descriptor(currentDescriptor.InputPosition, newGSSVertex, edge.NonTerminalSymbolStartState, None)
           |> addDescriptor
           positionsForPops
           |> ResizeArray.iter (fun matchedRange ->                   
               let rightSubRange =
                   MatchedRange(
                        matchedRange.InputRange.StartPosition
                      , matchedRange.InputRange.EndPosition
                      , currentDescriptor.RSMState
                      , edge.State
                      , RangeType.NonTerminal edge.NonTerminalSymbolStartState
                   )
                                                                               
               let leftSubRange = currentDescriptor.MatchedRange
               let newRange = matchedRanges.AddMatchedRange(leftSubRange, rightSubRange)                       
               Descriptor(matchedRange.InputRange.EndPosition, currentDescriptor.GSSVertex, edge.State, Some newRange) |> addDescriptor)
    )
    
    outgoingTerminalEdgesInRSM
    |> Array.iter (fun e1 ->
        outgoingTerminalEdgesInGraph
        |> Array.iter (fun e2 ->
            let graphEdge = unpackInputGraphTerminalEdge e2
            let rsmEdge = unpackRSMTerminalEdge e1
            if graphEdge.TerminalSymbol = rsmEdge.TerminalSymbol
            then
                let currentlyMatchedRange =
                    MatchedRange(
                        currentDescriptor.InputPosition
                        , graphEdge.Vertex
                        , currentDescriptor.RSMState
                        , rsmEdge.State
                        , RangeType.Terminal rsmEdge.TerminalSymbol)
                    
                let newMatchedRange = matchedRanges.AddMatchedRange (currentDescriptor.MatchedRange, currentlyMatchedRange)                        
                Descriptor(graphEdge.Vertex, currentDescriptor.GSSVertex, rsmEdge.State, Some newMatchedRange) |> addDescriptor))
\end{lstlisting}
